# Supplementary material for: Rapid hydrofracture of icy moon shells: insights from glaciology
Source: arXiv:2403.09888 source file (2025-02-06)
Supplement: Supplementary file 1 [file RL_supportinginformation.pdf]

**Rapid hydrofracture of icy moon shells: insights from glaciology**

Robert Law

University of Bergen, Bjerknes Centre for Climate Research

**Contents of this file**

Appendices A-D

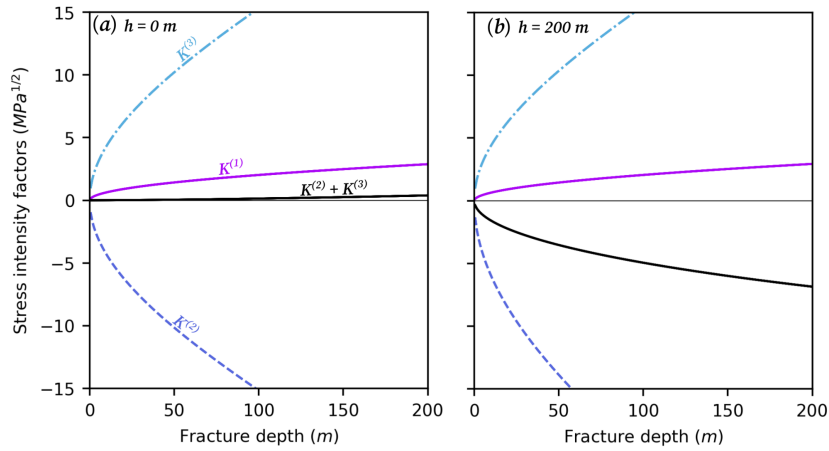

**Fig. S1:**  $K^{(1)}$ ,  $K^{(2)}$ ,  $K^{(3)}$  and  $K^{(2)} + K^{(3)}$  as fracture depth increases for  $h = 0$  m and  $h = 200$  m.  $a = 500$  m,  $H = 10$  km, and  $R_{xx} = 0.1$  MPa for both panels.

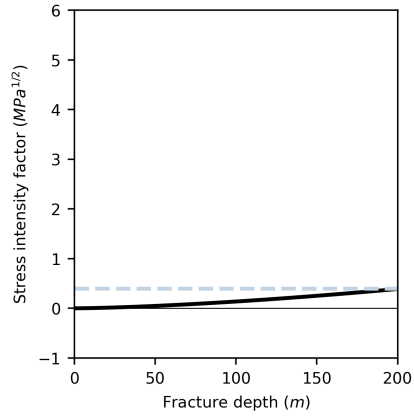

**Fig. S2:** Stress intensity factor under a tensile stress of 0 MPa with  $h = 0$ ,  $a = 0$ , and  $H = 30$  km.

### Text S1

Freeze onto a side wall,  $W$  (m) at time  $t$  (s) is calculated as

$$W(t) = \frac{2C(T_m - T_o)}{\sqrt{\pi L}} \sqrt{kt} \quad (\text{S1})$$

where  $C = 2093 \text{ J kg}^{-1} \text{ K}^{-1}$  is the specific heat,  $k = 1.18 \times 10^{-6} \text{ m}^2 \text{ s}^{-1}$  is the thermal diffusivity,  $L = 3.3 \times 10^5 \text{ J kg}^{-1}$  is the latent heat of ice,  $T_m$  is the melting point of ice, and  $T_o$  is the temperature of the ice wall ([Rubin, 1995](#); [Alley et al., 2005](#)).

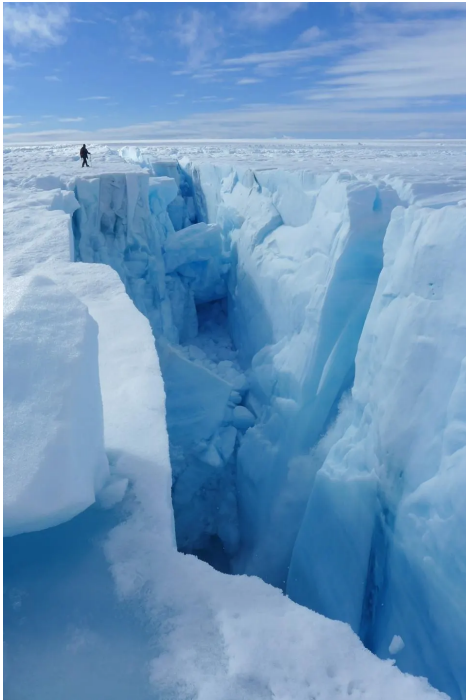

**Fig. S3:** The immediate aftermath of a supraglacial lake drainage at Sermeq Kujalleq (Store Glacier) in Greenland. Photo credit: Poul Christoffersen.
